# Supplementary material for: Reproducibility review of "Why Not Other Classes": Towards Class-Contrastive Back-Propagation Explanations
Source: arXiv:2501.11096 source file (2025-01-19)
Supplement: Supplementary file 1 [file Errors_in_the_original_paper.tex]

\section{Errors in the original paper}
