# Supplementary material for: Reproducibility review of "Why Not Other Classes": Towards Class-Contrastive Back-Propagation Explanations
Source: arXiv:2501.11096 source file (2025-01-19)
Supplement: Supplementary file 2 [file Revised_proof.tex]

\section{Revised proof}
